# Supplementary material for: Inference in Deep Gaussian Processes using Stochastic Gradient Hamiltonian Monte Carlo
Source: arXiv:1806.05490 source file (2018-11-12)
Supplement: Supplementary file 1 [file supplementary.pdf]

# A Static Mean function

Following the suggestion of Salimbeni and Deisenroth [2017], we added a static mean function to the output of each hidden layer. The static mean function helps to avoid degenerate covariance matrices. The static mean function is the identity $\boldsymbol{x} \mapsto \boldsymbol{I}\boldsymbol{x}$ unless the dimensionality of the output is lower than the input, in which case the static mean function is derived using the Singular-Value Decomposition $\boldsymbol{x} \mapsto \boldsymbol{V}^T\boldsymbol{x}$ where $\boldsymbol{x} = \boldsymbol{V}\boldsymbol{D}\boldsymbol{V}^T$ with $\boldsymbol{D}$ being a diagonal matrix of the size of the dimensionality of the output.

Moreover, the inducing inputs, which are sensitive to initialization [Turner and Sahani, 2011], can be initialized by propagating randomly selected datapoints through the static mean function of each layer.

# B Decoupled Deep Gaussian Processes

This section describes the approach of Cheng and Boots [2017] for single layer GPs followed by our generalization to DGPs along with an evaluation of different parameterizations that are necessary to stabilize convergence for DGPs.

In the single layer GP, the posterior mean $\tilde{\mu}$ and covariance $\tilde{\Sigma}$, referring to $q(\boldsymbol{f}|\boldsymbol{m}, \boldsymbol{S}) = \mathcal{N}(\boldsymbol{f}|\tilde{\mu}, \tilde{\Sigma})$, are parameterized by $\boldsymbol{m}$ and $\boldsymbol{S}$ where $q(\boldsymbol{u}) = \mathcal{N}(\boldsymbol{u}|\boldsymbol{m}, \boldsymbol{S})$. In the decoupled version, a new parameterization is used that utilizes two different sets of inducing inputs $\boldsymbol{Z}_a$ and $\boldsymbol{Z}_b$. $\tilde{\mu}$ is parameterized using the substitution $\boldsymbol{a} = K^{-1}_{\boldsymbol{Z}_a\boldsymbol{Z}_a}\boldsymbol{m}$ (Eq. 1). This is appealing because it does not require the computation of the inverse covariance matrix $K^{-1}_{\boldsymbol{Z}_a\boldsymbol{Z}_a}$ to calculate $\tilde{\mu}$. $\tilde{\Sigma}$ is defined using $(\boldsymbol{B}^{-1} + K_{\boldsymbol{Z}_b\boldsymbol{Z}_b})^{-1} = K^{-1}_{\boldsymbol{Z}_b\boldsymbol{Z}_b}(K_{\boldsymbol{Z}_b\boldsymbol{Z}_b} - \boldsymbol{S})K^{-1}_{\boldsymbol{Z}_b\boldsymbol{Z}_b}$:

$$
\begin{aligned}
\tilde{\mu} &= K_{\boldsymbol{x}\boldsymbol{Z}_a}\boldsymbol{a} \\
\tilde{\Sigma} &= K_{\boldsymbol{x}\boldsymbol{x}} - K_{\boldsymbol{x}\boldsymbol{Z}_b}(\boldsymbol{B}^{-1} + K_{\boldsymbol{Z}_b\boldsymbol{Z}_b})^{-1}K^T_{\boldsymbol{x}\boldsymbol{Z}_b} \,.
\end{aligned} \tag{1}
$$

Given the new parameterization, the ELBO takes a slightly different form. The equations generalized to multiple layers take the form

$$
\begin{aligned}
\mathcal{L} =& \mathbb{E}_{q(\boldsymbol{f}_l)}\big[\log p(\boldsymbol{y}|\boldsymbol{f}_l)\big] - \sum_{l=1}^{L} \mathrm{KL}\big[q_l||p_l\big] \\
\mathrm{KL}\big[q_l||p_l\big] =& \frac{1}{2}\boldsymbol{a}_l^T K_{\boldsymbol{Z}_a\boldsymbol{Z}_a}\boldsymbol{a}_l + \frac{1}{2}\log|\boldsymbol{I} + K_{\boldsymbol{Z}_b\boldsymbol{Z}_b}\boldsymbol{B}_l| \\
& - \frac{1}{2} tr\big(K_{\boldsymbol{Z}_b\boldsymbol{Z}_b}(\boldsymbol{B}_l^{-1} + K_{\boldsymbol{Z}_b\boldsymbol{Z}_b})^{-1}\big)
\end{aligned} \tag{2}
$$

where the KL divergence is given up-to a constant.

The reformulation greatly reduces the computational complexity. The time complexity of calculating the output mean in a single layer is $O(M^3 + NM)$, the output variance is $O(M^3 + NM^2)$ and the KL divergence is $O(M^3 + NM^2)$ where $M$ is $|\boldsymbol{Z}|$ and $N$ is the size of the minibatch. However, after the decoupling, the cost of computing the output mean becomes $O(NM_a)$, the variance becomes $O(NM_b^2 + M_b^3)$ and the KL divergence becomes $O(NM_a + NM_b^2 + M_b^3)$ per layer. This is due to the new parameterization not requiring the costly inversion of the covariance matrix $K^{-1}_{\boldsymbol{Z}_a\boldsymbol{Z}_a}$ when computing the predictive mean. The overall cost reduces from $O\big(L(DNM^2 + M^3)\big)$ to $O\big(L(DNM_a + DNM_b^2 + M_b^3)\big)$ where $L$ is the number of layers and $D$ is the width of the hidden layers. Note that the cost of inverting the covariance matrix does not scale with the layer width, since every node in the same layer shares the same convariance matrix. This leads to considerable improvement in training time if $M_b < M$.

**Alternative parameterizations** Unfortunately, the parameterization advocated by Cheng and Boots [2017] (Eq. 1), referred as $\tilde{\mu}_{CB}$ and $\tilde{\Sigma}_{CB}$ onwards) has poor convergence properties. The dependencies of the values of $\boldsymbol{a}_l$ in the ELBO result in a highly non-convex optimization problem, which then leads to high variance gradients. This impedes convergence.

Table 1: Different parameterizations of the mean. $\boldsymbol{L}$ refers to the Cholesky-decomposition: $\boldsymbol{L}\boldsymbol{L}^T = K_{\boldsymbol{Z}_a\boldsymbol{Z}_a}$

| $\tilde{\mu}$, $\tilde{\Sigma}$ | Parameters | Complexity |
|---|---|---|
| $\tilde{\mu}_{CB} = K_{\boldsymbol{X}\boldsymbol{Z}_a} diag(K_{\boldsymbol{Z}_a\boldsymbol{Z}_a})^{-1}\boldsymbol{a}$<br>$\tilde{\Sigma}_{CB} = K_{\boldsymbol{X}\boldsymbol{X}} - K_{\boldsymbol{X}\boldsymbol{Z}_b}(\boldsymbol{B}^{-1} + K_{\boldsymbol{Z}_b\boldsymbol{Z}_b})^{-1}K^T_{\boldsymbol{X}\boldsymbol{Z}_b}$ | $\boldsymbol{a}, \boldsymbol{B}$ | $O\big(L(DNM_a)\big)$<br>$O\big(L(DNM_b^2 + M_b^3)\big)$ |
| $\tilde{\mu}_{GP} = K_{\boldsymbol{X}\boldsymbol{Z}_a}(\boldsymbol{L}^T)^{-1}\boldsymbol{m}$<br>$\tilde{\Sigma}_{GP} = K_{\boldsymbol{X}\boldsymbol{X}} - K_{\boldsymbol{X}\boldsymbol{Z}_b}K^{-1}_{\boldsymbol{Z}_b\boldsymbol{Z}_b}(K_{\boldsymbol{Z}_b\boldsymbol{Z}_b} - \boldsymbol{S})K^{-1}_{\boldsymbol{Z}_b\boldsymbol{Z}_b}K^T_{\boldsymbol{X}\boldsymbol{Z}_b}$ | $\boldsymbol{m}, \boldsymbol{S}$ | $O\big(L(DNM_a + M_a^3)\big)$<br>$O\big(L(DNM_b^2 + M_b^3)\big)$ |

Using the substitution $K^{-1}_{\boldsymbol{Z}_b\boldsymbol{Z}_b}(K_{\boldsymbol{Z}_b\boldsymbol{Z}_b} - \boldsymbol{S})K^{-1}_{\boldsymbol{Z}_b\boldsymbol{Z}_b} = (\boldsymbol{B}^{-1} + K_{\boldsymbol{Z}_b,\boldsymbol{Z}_b})^{-1}$ in equation 1 we obtain formulas for the mean and the variance ($\tilde{\mu}_{GP}$, $\tilde{\Sigma}_{GP}$) shown in Table 1.For the mean, we precondition $\boldsymbol{m}$ with $\boldsymbol{L}^{-1}$, the inverse Cholesky factor of $K_{\boldsymbol{Z}_a\boldsymbol{Z}_a} = \boldsymbol{L}\boldsymbol{L}^T$. The motivation for the preconditioner is that it transforms the prior distribution to be a standard Gaussian with mean 0 and covariance $\boldsymbol{I}$. This aids convergence, because the term for the mean in the ELBO (Eq. 2) $\frac{1}{2}\boldsymbol{m}_l^T K^{-1}_{\boldsymbol{Z}_a\boldsymbol{Z}_a}\boldsymbol{m}_l$ simplifies to $\frac{1}{2}\boldsymbol{m}_l'^T\boldsymbol{m}_l'$.

As discussed earlier, $\tilde{\mu}_{CB}$ shows unstable convergence. While the problem is fixed with $\tilde{\mu}_{GP}$, this comes at a cost. Both of the these require computing the inverse covariance matrix for the mean ($K^{-1}_{\boldsymbol{Z}_a\boldsymbol{Z}_a}$), which leads to an increased overall cost of $O\big(L(DNM_a + M_a^3 + DNM_b^2 + M_b^3)\big)$. Fortunately, this is still an improvement over the original cost of DGPs when $N$ and $D$ are large and $M_b < N$, due to the term $LDNM_b^2$ dominating the overall cost. In our experiments, we used $\tilde{\mu}_{GP}$.

In our experiments, the decoupling slightly improved the performance compared to DGPs with DSVI on the regression datasets and it had a significant impact on the MNIST dataset.

# References

C.-A. Cheng and B. Boots. Variational Inference for Gaussian Process Models with Linear Complexity. *ArXiv e-prints*, Nov. 2017.

H. Salimbeni and M. Deisenroth. Doubly Stochastic Variational Inference for Deep Gaussian Processes. *ArXiv e-prints*, May 2017.

R. E. Turner and M. Sahani. Two problems with variational expectation maximisation for time-series models. 2011.
